# Supplementary material for: GraphMoRE: Mitigating Topological Heterogeneity via Mixture of Riemannian Experts
Source: arXiv:2412.11085 source file (2024-12-15)
Supplement: Supplementary file 1 [file checklist.tex]

\section*{Reproducibility Checklist}
\begin{enumerate}
    \item This paper:
    \begin{itemize}
        \item Includes a conceptual outline and/or pseudocode description of AI methods introduced. {\color{blue}[Yes]} See Algorithm~\ref{alg}.
        \item Clearly delineates statements that are opinions, hypothesis, and speculation from objective facts and results. {\color{blue}[Yes]}
        \item Provides well marked pedagogical references for less-familiare readers to gain background necessary to replicate the paper. {\color{blue}[Yes]} See Sec~\ref{sec:Preliminary}.
    \end{itemize}

    \item Does this paper make theoretical contributions? If yes, please complete the list below. {\color{orange}[No]}
    \begin{itemize}
        \item All assumptions and restrictions are stated clearly and formally. {\color{gray}[N/A]}
        \item All novel claims are stated formally (e.g., in theorem statements). {\color{gray}[N/A]}
        \item Proofs of all novel claims are included. {\color{gray}[N/A]}
        \item Proof sketches or intuitions are given for complex and/or novel results. {\color{gray}[N/A]}
        \item Appropriate citations to theoretical tools used are given. {\color{gray}[N/A]}
        \item All theoretical claims are demonstrated empirically to hold. {\color{gray}[N/A]}
        \item All experimental code used to eliminate or disprove claims is included. {\color{gray}[N/A]}
    \end{itemize}

    \item Does this paper rely on one or more datasets? If yes, please complete the list below. {\color{blue}[Yes]}
    \begin{itemize}
        \item A motivation is given for why the experiments are conducted on the selected datasets. {\color{blue}[Yes]} See Sec~\ref{sec:exp_Datasets} and Appendix~\ref{sec:datasets}.
        \item All novel datasets introduced in this paper are included in a data appendix. {\color{gray}[N/A]} 
        \item All novel datasets introduced in this paper will be made publicly available upon publication of the paper with a license that allows free usage for research purposes. {\color{gray}[N/A]}
        \item All datasets drawn from the existing literature (potentially including authors’ own previously published work) are accompanied by appropriate citations. {\color{blue}[Yes]}
        \item All datasets drawn from the existing literature (potentially including authors’ own previously published work) are publicly available. {\color{blue}[Yes]}
        \item All datasets that are not publicly available are described in detail, with explanation why publicly available alternatives are not scientifically satisficing. {\color{gray}[N/A]}
    \end{itemize}

    \item Does this paper include computational experiments? If yes, please complete the list below. {\color{blue}[Yes]}
    \begin{itemize}
        \item Any code required for pre-processing data is included in the appendix. {\color{blue}[Yes]}
        \item All source code required for conducting and analyzing the experiments is included in a code appendix. {\color{blue}[Yes]}
        \item All source code required for conducting and analyzing the experiments will be made publicly available upon publication of the paper with a license that allows free usage for research purposes. {\color{blue}[Yes]}
        \item All source code implementing new methods have comments detailing the implementation, with references to the paper where each step comes from. {\color{blue}[Yes]}
        \item If an algorithm depends on randomness, then the method used for setting seeds is described in a way sufficient to allow replication of results. {\color{blue}[Yes]}
        \item This paper specifies the computing infrastructure used for running experiments (hardware and software), including GPU/CPU models; amount of memory; operating system; names and versions of relevant software libraries and frameworks. {\color{blue}[Yes]} See Appendix~\ref{Sec:RunningEnvironment}.
        \item This paper formally describes evaluation metrics used and explains the motivation for choosing these metrics. {\color{blue}[Yes]} See Appendix~\ref{Sec:Exp_DownstreamTasks}.
        \item This paper states the number of algorithm runs used to compute each reported result. {\color{blue}[Yes]} See Sec~\ref{sec:setting}.
        \item Analysis of experiments goes beyond single-dimensional summaries of performance (e.g., average; median) to include measures of variation, confidence, or other distributional information. {\color{blue}[Yes]}
        \item The significance of any improvement or decrease in performance is judged using appropriate statistical tests (e.g., Wilcoxon signed-rank). {\color{orange}[No]}
        \item This paper lists all final (hyper-)parameters used for each model/algorithm in the paper’s experiments. {\color{blue}[Yes]} See Appendix~\ref{Sec:Hyperparameters} and Appendix~\ref{Sec:Details}.
        \item This paper states the number and range of values tried per (hyper-) parameter during development of the paper, along with the criterion used for selecting the final parameter setting. {\color{blue}[Yes]} See Appendix~\ref{Sec:Hyperparameters}.
    \end{itemize}
\end{enumerate}
